# Supplementary material for: Patchwork: A Polyhedral Implicit Representation for Highly Detailed 3D Shapes
Source: arXiv:2605.16266 source file (2026-11-25)
Supplement: Supplementary file 1 [file fig_supp_failure_cases.tex]

\setlength{\cmpimgw}{0.3\linewidth}
\setlength{\cmpspace}{\dimexpr(\linewidth - 3\cmpimgw)/2\relax}
\setlength{\cmplabelw}{\dimexpr\linewidth/3\relax}

\renewcommand{\cmprow}[2]{%
  \cmpimg{#1}{#2}{ablation_geo_init}\cmpsep
  \cmpimg{#1}{#2}{ours2}\cmpsep
  \cmpimg{#1}{#2}{gt}
}

\begin{figure*}[t]
\centering

\cmprow{failure_cases}{70558}
\cmprow{failure_cases_cut_open}{70558}
\cmprow{failure_cases}{103354}
\cmprow{failure_cases_cut_open}{103354}

%\vspace{-0.5pt}
% \cmprow{thingi10k}{316358}
\vspace{-10pt}\hrule\vspace{3pt}
%\vspace{-0.5pt}\hrule\vspace{0.5pt}

\cmplabelsfailure

\caption{Some failure cases showing the limitations of our method.}
\label{fig:supp_failure_cases}

\end{figure*}
